# Supplementary material for: Polymeric jets throw light on the origin and nature of the forest of solar spicules
Source: arXiv:2211.04493 source file (2022-11-08)
Supplement: Supplementary file 1 [file supplementary.pdf]

## SUPPLEMENTARY MATERIAL: POLYMERIC JETS AND SOLAR SPICULES

### 1. Comparison of viscoelastic and Maxwell stresses

In a polymeric fluid, the polymer not just stretches in the flow direction but in the process also exerts a stress back on the fluid which acts to suppress the fluid turbulence. In order to quantify this back reaction, we can compare the strength of the two different terms in the Navier-Stokes equation, namely, the viscoelastic stress and the inertial stress on the fluid. Further, to motivate the polymeric fluid-MHD analogy we compare this ratio for a polymeric fluid with the corresponding ratio of the Maxwell's stress to inertial stress for the case of solar MHD. A similar exercise was carried out by [1] assuming the Oldroyd-B model[2] of an incompressible viscoelastic fluid of uniform density, $\rho$, a polymer viscosity, $\eta_p$, and relaxation time, $\tau$. The Oldroyd-B is a linear polymer model– viscosity $\propto$ strain rate– which is valid under two conditions, namely: i) dilute polymer solution i.e., concentrations at which polymer chain-chain interactions are negligible and; ii) the polymer chain is infinitely extensible. Even though we observe jetting behaviour in a wide range of polymer concentrations, some of which lie outside the strict validity of the Oldroyd-B, we shall consider only those experiments with Poly Ethylene Oxide (PEO) where the polymer concentration is dilute enough to enable a direct comparison in this section. A major difference with [1, 3, 4] is that we use an elongational geometry applicable to jets rather than Couette flow geometry which is applicable to elasto-rotational instability (ERI). The stress tensor components in the case of uniaxial incompressible extensional flow (filamentary, Supplementary Fig.1) in 3-dimensions corresponding to the velocity field given by, $u_x = -x\dot{\epsilon}/2$, $u_y = -y\dot{\epsilon}/2$ and $u_z = z\dot{\epsilon}$ can be written as (Chap 5 of [5]),

$$\sigma_{xx} = \sigma_{yy} \tag{1}$$

$$\sigma_{zz} - \sigma_{xx} = \dot{\epsilon}\eta_E(\dot{\epsilon}) \tag{2}$$

$$\sigma_{xy} = \sigma_{yz} = \sigma_{xz} = 0 \tag{3}$$

where, $\dot{\epsilon}$ is the strain rate and $\eta_E$ is the uniaxial extensional viscosity. The traceless stress tensor, $[\sigma_{ij}]$, can then be given by,

$$\overleftrightarrow{\sigma} = \frac{\mathrm{Tr}\eta_p}{3}\begin{bmatrix} -\dot{\epsilon} & 0 & 0 \\ 0 & -\dot{\epsilon} & 0 \\ 0 & 0 & 2\dot{\epsilon} \end{bmatrix} \tag{4}$$

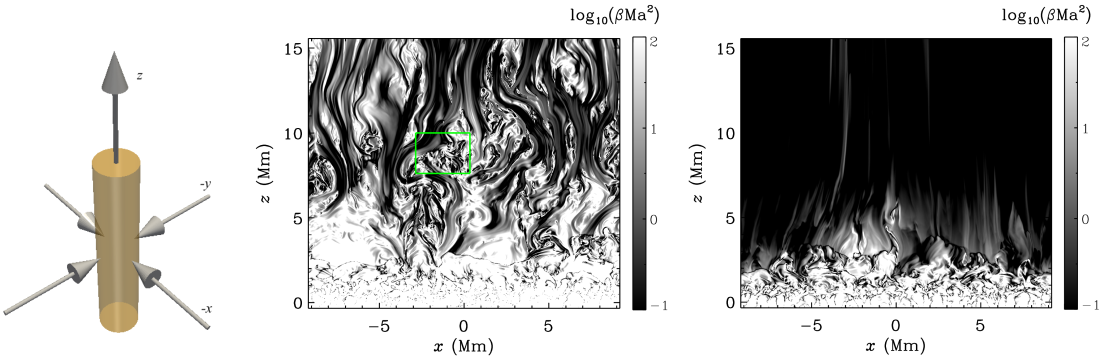


Supplementary Figure 1. *Left panel*: An example of a uniaxial extensional flow field. *Middle panel*: logarithm of the quantity $\beta \mathrm{Ma}^2$ for imposed vertical magnetic field $B_{\mathrm{imp}} = 0.1\,\mathrm{G}$. The green square shows the region for which the root-mean-square of velocities have been calculated in the text. *Right panel*: same as the middle panel but for $B_{\mathrm{imp}} = 1\,\mathrm{G}$.

where, Tr is the Trouton ratio defined as

$$\mathrm{Tr} = \frac{\eta_E(\dot{\epsilon})}{\eta_p} \tag{5}$$

where, $\eta_p = \lim_{\dot{\epsilon}\to 0} \eta_E(\dot{\epsilon})$ is the viscosity of the polymer subjected to shearing flows as measured in our case by the Anton-Paar MCR 302 rheometer. For a Newtonian fluid, $\mathrm{Tr} = 3$, whereas for dilute aqueous polymers such as polyethylene oxide (PEO) this ratio can be as large as $10^4$ depending on $\dot{\epsilon}$. Even though in the case of Faraday excitation we have a periodic driver, yet in the absence of any detail knowledge of the functional form of the flow inside the jet, we have made the drastic assumption that the flow is quasi-steady during the rise time of the jet, like in the case of the filamentary flow in a capillary breakup rheometry (CABER) set-up.

On the other hand the Maxwell's stress tensor is given by,

$$\mathcal{M}_{ij} = \frac{B_i B_j}{\mu_0} - \frac{B^2}{2\mu_0}\delta_{ij}. \tag{6}$$

In our case of a 2-dimensional set-up with $B_y = 0$, $\partial/\partial y \to 0$, and non-zero magnetic fields only in the $[x, z]$-plane, the stress tensor has a simple form given by,

$$\overleftrightarrow{\mathcal{M}} = \frac{1}{2\mu_0}\begin{bmatrix} B_x^2 - B_z^2 & 0 & 2B_xB_z \\ 0 & -B_x^2 - B_z^2 & 0 \\ 2B_xB_z & 0 & B_z^2 - B_x^2 \end{bmatrix}. \tag{7}$$

Since the $y$-coordinate is trivial, the trace of the reduced $2\times 2$ matrix is $\mathcal{M}_{11}+\mathcal{M}_{33}=0$. The $3\times 3$ Maxwell's stress tensor has the following eigenvalues,

$$\lambda_{1,2} = -\frac{B_x^2+B_z^2}{2\mu_0}, \lambda_3 = \frac{B_x^2+B_z^2}{2\mu_0}. \tag{8}$$

Invoking the similarity of the equation of motion for a viscoelastic fluid and MHD *i.e.*, Eqs. 2.2 and 2.5 from [1], we can arrive at the following analogy between the anisotropic stress terms in either system. Namely, comparing Eqs. 4 and 8 we have,

$$\lambda_3 \leftrightarrow \sigma_{zz} \tag{9}$$

$$\text{Or, } \frac{B_x^2+B_z^2}{2\mu_0} \leftrightarrow \frac{2\mathrm{Tr}(c)\eta_p(c)\dot{\epsilon}}{3}. \tag{10}$$

Note that $\eta_p = \rho\nu_p$, where, $\nu_p$ is the kinematic viscosity of the polymeric fluid and we expect it to be also a function of the concentration, $c$. Also, $\beta = c_s/v_A$, is the plasma-$\beta$ and $Ma = u/c_s$, is the Mach number of the plasma flow. We scale the stress terms with the inertial stress represented approximately as the square of the fluid velocity in both cases and compare $\beta^{-1}Ma^{-2}$ (MHD) to $2\mathrm{Tr}\nu_p/(3u_zL)$ (polymeric fluid). In Supplementary Figs. 1b, c, we show the variation of the quantify $\beta\mathrm{Ma}^2$ for $B_{\mathrm{imp}} = 0.1, 1\,\mathrm{G}$, respectively. It is clear from comparing the two panels of this figure with panels of Fig. 1c in the main text that in regions where $\beta^{-1}Ma^{-2} > 1$ are the regions where formation of Kelvin-Helmholtz vortices are suppressed. Although, we do not have an idea of the exact value of Tr, but, intuitively it must depend on the concentration $c$ and experimentally known to be in the range $3 < \mathrm{Tr} < 10^4$ for polymers like PEO. For high molecular weight PEO solutions with $Oh > 1$, Trouton ratios of $\mathrm{Tr} > 10^3$ are known to be realized [6]. Let us use the measured value of $\nu_p = 9.8\pm 0.1\times 10^{-7}\ \mathrm{m^2\,s^{-1}}$ for 100 ppm PEO solution, and $\dot{\epsilon} \sim u_z/L$, where $u_z \sim 0.2\,\mathrm{m\,s^{-1}}$ is the typical tip velocity of the jet and $L \sim 0.02\,\mathrm{m}$ is the maximum height of the jet in Fig.1d. Using the above values the non-dimensional viscoelastic stress, $10^{-3} \ll 2\mathrm{Tr}(c)\nu_p(c)/(3u_zL) < 3$. Therefore, even though the two systems are widely different, and in spite of several approximations, it is surprising that the relative strengths of stresses seem comparable.

## 2. Threshold magnetic field for suppression of Kelvin-Helmholtz instability

The panel (e) of Fig. 1 shows an initial monotonic decrease of vortices detected with increasing the magnetic field, $B_z$, before the curve goes to saturation with no vortices detected. In the Methods section, we also indicate that the algorithm for detection of vortices assumes that the rotation velocity is larger than the expansion or contraction velocity or that circular vortices ($|v_x| \sim |v_z|$) are more likely to be detected. Analysis of the velocity components inside a small region denoted by the green rectangle in Fig. 1b gives a value of $|v_x| \sim 1.06|v_z|$ (for $B_{\mathrm{imp}} = 0.1\,\mathrm{G}$ and numerous vortices) and $|v_x| \sim 0.11|v_z|$ (for $B_{\mathrm{imp}} = 1.0\,\mathrm{G}$ and very few vortices). Also, note that in Extended Data Fig. 2b, where the horizontal velocity is damped artificially in a 2D solar atmospheric set-up without any imposed vertical magnetic field, the KH vortices are suppressed and we obtain a forest of

vertical jets. Let us assume that $|B_x| \sim |B_z|\delta$, with $\delta < 1$ for a dominant vertical field. Focussing on the contribution of the magnetic field, we can write the $x$-component of the velocity equation assuming only the Lorentz force in the right hand side as,

$$\frac{\partial v_x}{\partial t} = \frac{B_z^2 \tau}{\rho \mu_0} \nabla^2 v_x + \frac{v_x B_z \tau}{\mu_0 \rho} \nabla^2 B_z + \text{other terms of order } \delta. \tag{11}$$

To arrive at the above equation, we have additionally used the induction equation (integrated over a time scale $\tau$) to rewrite terms involving $\partial B_x/\partial z$ and $\partial B_z/\partial x$. We note that the first term has the form of a diffusion term and serves to decrease $v_x$ and, further, ignore the second term in Eq. 11 as an approximation. Let the shear rate $(dv_z/dx)$ produced as a result of vertical wave driving at the edge of an initial vertical jet be $\sim v_z/d$, where, $d$ is the width of the jet. We take $\tau$ also to be the inverse of the shear rate. The diffusion time for $v_x$ must be shorter than the shearing time, for the vortices to elongate vertically from their circular cross section, and no longer be detected, *i.e.,* $|v_x| < |v_z|$. This implies,

$$\frac{B_z^2}{\rho \mu_0 v_z d} > \frac{v_z}{d} \tag{12}$$

Let the Alfvén velocity in the vertical direction be $v_{Az} = B_z/\sqrt{\mu_0 \rho}$, the plasma beta, $\beta = c_s^2/v_{Az}^2$, and the Mach number, $Ma = v_z/c_s$. Then, Eq. 12 can be rearranged to show that in regions where $\beta Ma^2 < 1$, the vortex formation by the shear instability will be suppressed.

## 3. Threshold concentration for suppression of Plateau-Rayleigh instability

In analogy with panel (e) of Fig. 1, panel (f) also indicates that the number of droplets ejected in the experiments decrease with increasing polymer concentration and then goes to zero for concentrations above 50 ppm. This points to the existence of a threshold of polymer concentration beyond which the Plateau-Rayleigh instability[7] is effectively arrested.

The physical model of the polymer chains in the fluid responding to a flow is as described by [8], and Chap 20 of [9]. A rigorous analytical treatment (*i.e.*, by using Langevin dynamics) is non-trivial and depends on microscopic details of the forcing function induced by the flow on beads of a particular polymer chain, *e.g.*, uniform (non uniform) and steady (oscillatory) forcing along its partially coiled length. However, using the macroscopic description that the polymer chains are microscopic springs associated with a single spring constant, and embedded in the fluid responding to and reacting on the jetting flow, we can easily motivate the existence of a threshold concentration.

Without going into the exact spatial profile of the flow inside a jet and an associated mathematically exact analysis, we make certain approximations for calculating the threshold polymer concentration: i) the applied stress is almost constant during the rise phase of the jet; ii) the Maxwell's pot model where there are $\sim c$ springs and pots per unit volume of the fluid (a measure of polymer concentration) each of which can store an energy $E_p$. In an extensional flow, these elastic springs would absorb energy from the flow and during

the relaxation, the energy would be dissipated in the pots. This spring constant depends on the molecular weight and structure of the chain. For a given Faraday amplitude and frequency, let the velocity of a vertical jet (of length, $L$, and width, $d$) ejected be $v_0$ for a non-polymeric fluid. In the presence of extensible polymeric coiled chains, let the corresponding jet velocity be denoted as $v_1$. And, $\dot{\epsilon} =\sim v_1/L$ be the strain rate and $\tau$ is the rise time of the jet. The viscous dissipation due to the kinematic extensional viscosity, $\nu_E$, is $\sim \rho\nu_E\dot{\epsilon}^2\tau/2$. Then, we can write

$$cE_p = \rho\nu_E\frac{v_1}{L} \tag{13}$$

and,

$$\frac{\rho}{2}(v_0^2 - v_1^2) = \frac{\rho\nu_E}{2}\dot{\epsilon}^2\tau. \tag{14}$$

In the absence of polymers, we expect the jet to have enough energy to overcome surface tension and produce at least a droplet. Therefore, $v_0^2 > 2n\gamma A/\rho V$, where A is the surface area of the droplet, $n$ is the number of droplets the jet disintegrates into, $V$ is the volume of the jet and $\gamma$ is the surface tension. Upon addition of a small quantity of polymer, the jet no longer has the extra energy to produce even a single droplet. Thus, $v_1^2 < 2\gamma A/\rho V$. By using Eq. 14 along with the first inequality involving $v_0$ we have,

$$v_1^2 + \frac{2cE_p}{\rho} > \frac{2n\gamma A}{\rho V} \tag{15}$$

and after rearrangement, for a cylindrical jet, we find a threshold for the polymer concentration, $c$, given by,

$$c > \frac{\rho v_1^2}{2E_p}\left(\frac{8n\gamma}{\rho v_1^2 L} - 1\right) > 0. \tag{16}$$

Most jets in the Faraday experiment, performed at 30 Hz with water, break into $n > 2$ droplets. Using guiding values from the identical experiment with 100 ppm PEO solution prepared using PEO of molecular weight, $M_w[\mathrm{PEO}] = 5000\,\mathrm{kg\,mol^{-1}}$, we can further calculate, $c \sim 10^{19}$ chains $\mathrm{m^{-3}}$. Substituting the typical measured values of $v_1 \sim 0.2\,\mathrm{m\,s^{-1}}$, $\gamma = 0.07\,\mathrm{N\,m^{-1}}$, $L = 0.02\,\mathrm{m}$ in Eq. 16 leads to $E_p > 8\times10^{-19}$ J, which is roughly the energy absorbed by each coiled polymer chain molecule. The typical size of a coiled polymer consisting of $N_p = M_w[\mathrm{PEO}]/M_w[C_2H_4O] \sim 113000$ monomers is given by $R_g \sim 1.3\sqrt{N_p}$ Å$\sim$ 440 Å, where 1.3 Å is the size of $C_2H_4O$ – the PEO monomer. In addition to this, we can assume a spring constant of $k = 3k_BT/R_g^2$, with the Boltzmann constant denoted, $k_B$, and $T = 300\,\mathrm{K}$. The extensional flow, during the rise phase of the jet, can uncoil the chain to $\sqrt{E_p/k} \sim 8$ times the coiled size $R_g$. There is of course a statistical distribution of energy and extension felt by the polymer molecules in the jet, but here we crudely assume that all polymer molecules absorb the same energy. Further, from Eq. 13, we obtain an estimate for the Trouton ratio, Tr, using the measured value for $\nu_p = 9.8\times10^{-7}\,\mathrm{m^2\,s^{-1}}$, namely,

$$\mathrm{Tr} = \frac{\nu_E}{\nu_p} > \frac{2v_1L}{\nu_p}\left(\frac{8n\gamma}{\rho v_1^2 L} - 1\right) \sim 3200. \tag{17}$$

The above value lies in the range quoted at the end of §1. Using the above analysis along with experimentally observed properties, like threshold concentration, height, width and velocity of jets, we are able to derive some reasonable order-of-magnitude numbers regarding the behaviour of polymer chains in a typical jet formed by Faraday excitation (*i.e.*, $E_p$, the energy absorbed by each chain, stretched chain length, Trouton number). This gives us confidence that some aspects of this highly non-linear system can still be understood from such a simple physics based approach.

## 4. Determination of $A_{\rm min}$

In this section, we provide a detailed explanation of the process followed to determine the threshold acceleration, $A_{\rm min}$ in Figs. 1a-b. We arrive at the plotted data points corresponding to minimum acceleration, $A_{\rm min}$, at any given frequency, denoted by filled triangles, by performing a sequence of independent runs sampling the vertical acceleration. An imaginary line connecting these filled triangles is the curve of $A_{\rm min}$ versus $f_0$ which is the approximate boundary in phase space where the forest of jets criteria starts to apply. In the range of discrete frequencies explored between 3-9 mHz (solar atmosphere) and 15-120 Hz (fluid), therefore the $A_0$–$f_0$ phase space is separated by the boundary defined by the data points into two regions–one in which a forest of jets are observed (at and above the data points denoted by filled symbols) and one where our forest of jet criteria is not satisfied (the data points denoted by open symbols). Therefore the transition from a forest to no forest lies somewhere in between the least acceleration filled and highest acceleration open triangles for these frequencies. This process is followed for all the frequencies but the vicinity of the transition is represented in the figure at three indicative frequencies, namely, 3.3, 5.5, and 7 mHz (Fig. 1a for solar atmosphere) and 20, 50, and 105 Hz (Fig. 1b for polymeric fluid) so as to sample the regions R1, R2 and R3. For an illustration of our method of arriving at data points used in Fig 1a, we provide at the 3.3 mHz driving frequency a Supplementary Video 9 (part I) of wave driving of the solar atmosphere. This driver corresponds to a vertical velocity amplitude of 0.50 km s$^{-1}$ (panel a) and 0.35 km s$^{-1}$ (panel b). Here, several jets, as characterized by synthetic Si IV emission using an analytical function (see Methods), reach heights $\geq$ 7 Mm during ten oscillation periods, after the nonlinear development phase, thereby satisfying the forest of jets criteria. Let us compare this to a driving amplitude of 0.25 km s$^{-1}$ (panel c), where five jets, still strongly resembling the driving profile and therefore no nonlinear development, are also seen but reaching heights $<$ 7 Mm during ten periods, thereby failing to satisfy the forest of jets criteria.

Likewise, for Fig 1b, we provide at the 50 Hz driving frequency a supplementary video 9 (part II). There, a Faraday excitation runs of 500 ppm PEO solution, corresponding to different vertical peak harmonic accelerations are performed. For a peak acceleration of $4.3g_{\rm E}$, four jets reach $\geq$ 0.5 cm length (1.3 cm mark on the scale in the Supplementary Video 9) in ten oscillation periods, again after the onset of nonlinear development phase indicated by the central jet ejection, and this threshold data point is recorded. Next, with a reduced peak acceleration of both $3.6g_{\rm E}$ and $4.1g_{\rm E}$ yields no jet and two jets, respectively, in the same duration. Further, the variation in repeated measurement of threshold criteria,

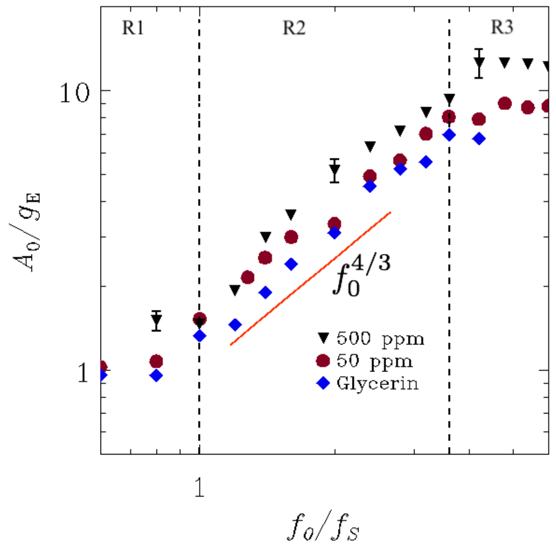


SUPPLEMENTARY FIGURE 2. The $A_0$–$f_0$ phase space to represent and compare the variation of threshold accelerations, $A_{\min}$ with driving frequency, $f_0$. Each filled symbol represents an independent experiment for different fluids, namely, 500 ppm (triangle), 50 ppm PEO (circle) solution and 55% glycerine (diamond). The error bars denote random variations obtained from repeated set of measurements at three different frequencies (20 Hz, 50 Hz and 105 Hz) for the 500 ppm PEO solution. The solid red line shows the $f_0^{4/3}$ dependence obtained for jets by dimensional arguments for a fluid under Faraday excitation[10].

performed at different times and with different batches of solutions, at three representative frequencies (20 Hz, 50 Hz and 105 Hz for 500 PEO in fluid experiments) are denoted by error bars (9%, 11% and 12%) in the Supplementary Fig. 2. For comparison with experiments with 500 ppm PEO, we also represent data points performed using the same technique as Fig. 1b but for different fluids, namely, 50 ppm PEO (lower polymer concentration and lower viscosity similar to water) and 55% glycerine solution (non-polymeric high viscosity similar to 1000 ppm PEO).

## REFERENCES

[1] Ogilvie, G. I. & Proctor, M. R. E. On the relation between viscoelastic and magnetohydrodynamic flows and their instabilities. *J. Fluid Mech.* **476**, 389–409 (2003).

[2] Oldroyd, J. G. On the formulation of rheological equations of state. *Proc. Roy. Soc. London* **200**, 523 (1950).

[3] Boldyrev, S., Huynh, D. & Pariev, V. Analog of astrophysical magnetorotational instability in a couette-taylor flow of polymer fluids. *Phys. Rev. E* **80**, 066310 (2009).

[4] Bai, Y., Crumeyrolle, O. & Mutabazi, I. Viscoelastic taylor-couette instability as analog of the magnetorotational instability. *Phys. Rev. E* **92**, 031001 (2015).
[5] Barnes, H., F., H. J. & Walters, K. *An introduction to rheology* (Elsevier, London, 1989).
[6] Dinic, J. & Sharma, V. Macromolecular relaxation, strain, and extensibility determine elastocapillary thinning and extensional viscosity of polymer solutions. *PNAS* **116**, 8766–8774 (2019).
[7] Plateau, J. A. F. Statique experimentale et theorique des liquides soumis aux seules forces moleculaires. *Paris: Gauthier Villars* **2** (1873).
[8] Marciano, Y. & Brochard-Wyart, F. Normal modes of stretched polymer chains. *Macromolecules* **28**, 985–990 (1995).
[9] Young, R.J., and Lovell, P.A. *Introduction to Polymers* (Elsevier, Boca Raton, 2011).
[10] Goodridge, C. L., Shi, W. T., Hentschel, H. G. E. & Lathrop, D. P. Viscous effects in droplet-ejecting capillary waves. *Phys. Rev. E* **56**, 472–475 (1997).
